# Supplementary material for: Non-convex online learning via algorithmic equivalence
Source: arXiv:2205.15235 source file (2022-10-12)
Supplement: Supplementary file 1 [file appendix.tex]

\section{Proof of Lemma~\ref{lem2}}\label{appendix}

\begin{proof}
We define the sequences $y^R_t, x^R_t$ as one step of OMD from our current iterate with learning rate $\eta$, i.e 
\begin{align*}
    y^R_{t+1} &= \nabla R^{-1}(\nabla R(x_t) - \eta \nabla f_t(x_t))\\
    x^R_{t+1} &= \argmin_{x\in \K} D_R(x||y^R_{t+1})
\end{align*}

Now, we note that $\nabla f_t(x_t)) = \frac{\nabla R(x_t)- \nabla R(y^R_{t+1})}{\eta}$ and hence, we have 
\begin{align*}
    \regret(\A) \le \sum_{t=1}^T \nabla f_t(x_t))^{\top}(x_t - x^{*}) &=\frac{1}{\eta}\sum_{t=1}^T (\nabla R(x_t)- \nabla R(y^R_{t+1}))^{\top} (x_t - x^{*})\\
    &= \frac{1}{\eta}\sum_{t=1}^T \big[D_R(x^{*}|| x_t) - D_R(x^{*}|| y^R_{t+1}) + D_R(x_t|| y^R_{t+1}) \big]\\
    & \le \frac{1}{\eta}\sum_{t=1}^T \big[D_R(x^{*}|| x_t) - D_R(x^{*}|| x^R_{t+1}) + D_R(x_t|| y^R_{t+1}) \big] 
\end{align*}
where the second equality follows via the three point lemma and the last inequality follows via projection. Now, we note that by the bound on $\|r_t\|_2$ and the Lipschitz condition on $D_R$, we have $|D_R(x^{*}|| x^R_{t+1}) - D_R(x^{*}|| x_{t+1})| =O( C G) $.  Combining with a telescoping argument, we have

\begin{align*}
    \regret(\A) &\le \frac{C T G}{\eta} + \frac{1}{\eta}\sum_{t=1}^T \big[D_R(x^{*}|| x_t) - D_R(x^{*}|| x_{t+1})\big] + \frac{1}{\eta}\sum_{t=1}^T D_R(x_t|| y^R_{t+1}) \\
    &\le \frac{C T G}{\eta} + \frac{D_R(x^{*}|| x_1)}{\eta} +\frac{1}{\eta}\sum_{t=1}^T D_R(x_t|| y^R_{t+1}) \le \frac{C T G}{\eta} + \frac{D}{\eta} +\frac{1}{\eta}\sum_{t=1}^T D_R(x_t|| y^R_{t+1})
\end{align*}
The final term is bounded via Cauchy-Schwartz:
\begin{align*}
    D_R(x_t|| y^R_{t+1}) + D_R(y^R_{t+1}|| x_t) &= (\nabla R(x_t)- \nabla R(y^R_{t+1}))^{\top}(x_t - y^R_{t+1})\\
    &= \eta \nabla f_t(x_t) ^{\top}(x_t - y^R_{t+1}) \\
    &\le \eta \|\nabla f_t(x_t)\|_2 \|x_t - y^R_{t+1}\|_2 \\
    &\le \frac{1}{2}\eta^2 \|\nabla f_t(x_t)\|^2_2 + \frac{1}{2}\|x_t - y^R_{t+1}\|^2_2 \\
\end{align*}
Noting that $D_R(y^R_{t+1}|| x_t) \ge \frac{1}{2}\|x_t - y^R_{t+1}\|^2_2$ via the $1$-strong convexity of $R$, we have $D_R(x_t|| y^r_{t+1}) \le \frac{1}{2}\eta^2 G^2$ by Assumption~\ref{assumption:bounds} and so 
\begin{align*}
    \regret \le \frac{C T G}{\eta} + \frac{D}{\eta} +\frac{\eta G^2 T}{2}~.
\end{align*}
\end{proof}

\section{Regret bound of the EG example}\label{sec:EG_app}
We modify the domain $\K$ to be the smoothed simplex with all weights being at least $T^{-\epsilon}$, where $\epsilon$ is to be determined later. The smoothing basically worsens the loss of each step by $O(G_F T^{-\epsilon})$, and in all worsens the regret by $O(G_F T^{1-\epsilon})$.

We need to check the constants in Assumption \ref{assumption:lipschitz} if they have dependence on $T$. The Lipschitzness of $q$ is fine, the $1-st$ derivative of $R$ and the Lipschitzness of $D_R(x\| \cdot)$ have only logarithmic dependence. However, the first and second derivatives of $q^{-1}$ and the third derivative of $R$ do have norms depending on $T$, with upper bounds to be $T^{\frac{\epsilon}{2}}$, $T^{\frac{3\epsilon}{2}}$ and $T^{2 \epsilon}$ respectively. 

As a result, we can only use $G=T^{2 \epsilon}$. Plugging it back to Lemma \ref{lem1}, we have that $C=O(T^{8 \epsilon} G_F^{\frac{3}{2}} \eta^{\frac{3}{2}})$. Combining this with Lemma \ref{lem2} we have that
$$
\regret(\A)=O(T^{10 \epsilon+1} G_F^{\frac{3}{2}} \eta^{\frac{1}{2}}+\frac{D}{\eta}+G_F T^{1-\epsilon})
$$
whenever $\eta<1$ which is the case. Balancing the first two terms give the optimal choice of $\eta=D^{\frac{2}{3}}G_F^{-1}T^{-\frac{20\epsilon+2}{3}}$. Then choosing $\eta=\frac{1}{23}$ gives an $O(T^{\frac{22}{23}})$ regret bound.
